# Supplementary material for: Characterizing Impacts of Heterogeneity in Federated Learning upon Large-Scale Smartphone Data
Source: arXiv:2006.06983 source file (2021-03-12)
Supplement: Supplementary file 1 [file appendices.tex]

\appendix
  
    \section{Olaf Configuration File}
        
        \begin{table}
          \caption{Description of the settings in Olaf's configuration file}
          \label{tab:config}
          \scalebox{0.9}{
          \begin{tabular}{llp{5cm}}
            \toprule
            Setting name&Type&Description\\
            \midrule
            config_name&String&the name of this configuration, same as the generated log's name\\
            dataset&String&dataset to use\\
            model&String&DL model to use, should implement the interface defined in \textit{model.py}\\
            num\_rounds&int&number of rounds to run, unlimited when num\_rounds < 0\\
            
          \bottomrule
        \end{tabular}}
        \end{table}
